# Supplementary material for: Enhanced Raman scattering of graphene using double resonance in silicon photonic crystal nanocavities
Source: arXiv:1806.02006 ancillary file (2018-06-06)
Supplement: Supplementary file 1 [file supplementary_material.pdf]

**Supplementary Material**

# Enhanced Raman scattering of graphene using double resonance in silicon photonic crystal nanocavities

W. Gomulya,[1, 2] H. Machiya,[2,3] K. Kashiwa,[4] T. Inoue,[4] S. Chiashi,[4] S. Maruyama,[4,5] and Y. K. Kato,[1, 2]

*[1)]Quantum Optoelectronics Research Team, RIKEN Center for Advanced Photonics, Saitama 351-0198, Japan*

*[2)]Nanoscale Quantum Photonics Laboratory, RIKEN Cluster for Pioneering Research, Saitama 351-0198, Japan*

*[3)]Department of Electrical Engineering, The University of Tokyo, Tokyo 113-8656, Japan*

*[4)]Department of Mechanical Engineering, The University of Tokyo, Tokyo 113-8656, Japan*

*[5)]Energy NanoEngineering Laboratory, National Institute of Advanced Industrial Science and Technology (AIST), Ibaraki 305-8564, Japan*

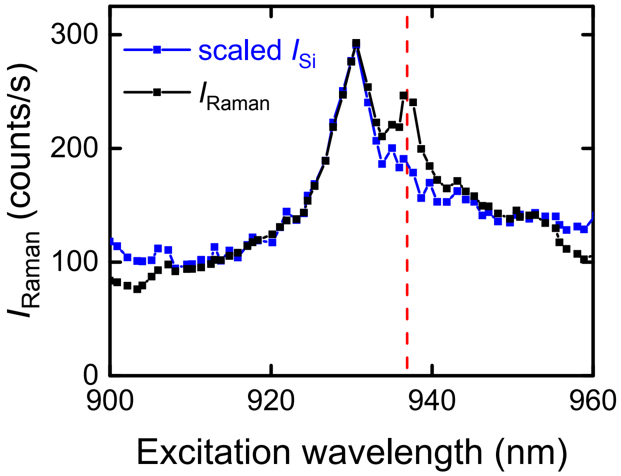


Fig. S1. Enhancement by the cavity mode. Raman excitation spectra (black) and scaled silicon PL peak intensity (blue) of the device shown in Fig. 4(a). The silicon PL peak intensity $I_{Si}$, which reflects the LGM spectrum, is scaled to match the spectral profile of the Raman peak intensity $I_{Raman}$ except for the enhancement due to the cavity mode at $\lambda_{ex} = 936$ nm (the red dashed line). The enhancement by the cavity mode is calculated by taking the ratio of $I_{Raman}$ and the scaled $I_{Si}$ at 936 nm, and we obtain an enhancement of 1.3.

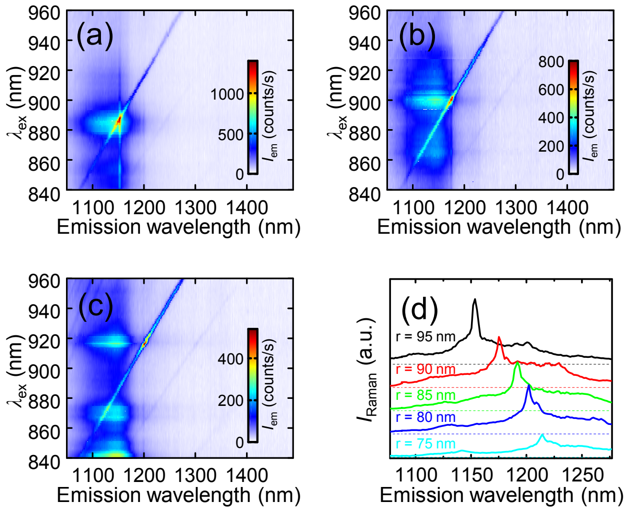


Fig. S2. Excitation spectroscopy maps for devices with $a = 355$ nm and (a) $r = 95$ nm, (b) $r = 90$ nm, (c) $r = 80$ nm. (d) Excitation spectra of the Raman peak intensity for devices with $a = 355$ nm and $r$ ranging from 75 nm to 95 nm. To fit the devices with $r = 90$ nm and $r = 95$ nm, we add another Lorentzian function to Eq. (1) for fitting the cavity mode. The curves are offset for clarity, and the dashed lines indicate zero intensities for each curve. The enhancement ratios by the double resonance with respect to the off-resonance Raman peak at 960 nm are 7.7, 5.9, 5.0, and 2.8 for the devices with $r = 90$ nm, 85 nm, 80 nm, and 75 nm, respectively. The enhancement for the device with $r = 95$ nm is not calculated because the Raman peak overlaps with the strong silicon PL enhanced by the LGM.
